# Supplementary material for: Proximal Gradient Algorithm with Momentum and Flexible Parameter Restart for Nonconvex Optimization
Source: arXiv:2002.11582 source file (2020-04-27)
Supplement: Supplementary file 1 [file supplementary.tex]

\clearpage
\appendix{
	\onecolumn
	{\centering\Large \textbf{Supplementary Materials}}

\section{Proof of \Cref{lemma: Acc-PGD dynamic}}

\LemmaDynamicPGD*

\begin{proof}
	The proof utilizes some intermediate results developed in \cite{Ghadimi2016b}, and we include the proof of these results for completeness of presentation. Throughout, we define ${\Gamma}_0 = 0, {\Gamma}_1 = 1, {\Gamma}_k = (1-{\alpha}_k) {\Gamma}_{k-1}$ for $k=2,3,...$. By the restarting nature of $\alpha_{k}$, it is easy to check that ${\Gamma}_k = 0$ whenever $k=Q_t$ for some $t$, and $\Gamma_{k}=\frac{2}{(k-Q_t)(k-Q_t+1)}$ otherwise. 
	
	Let the sequences $\{x_k\}_k, \{y_k\}_k, \{z_k\}_k$ be generated by \Cref{alg: Acc-PGD}. Let us first analyze a certain $(t-1)$-th restart period, which consists of the iterations $\{\ell: Q_{t-1}\le \ell \le Q_t-1\}$. We first bound the term $\|y_k - x_k\|$ for any iteration $k$ within this restart period. By the update rule of the momentum scheme in \Cref{alg: Acc-PGD}, we obtain that
	\begin{align}
	y_k - x_k &= z_{k-1} - \beta_{k-1} G_{\lambda_{k-1}}(x_{k-1}, \nabla f(z_{k-1})) - (x_{k-1} - \lambda_{k-1} G_{\lambda_{k-1}}(x_{k-1}, \nabla f(z_{k-1}))) \nonumber\\
	&= (1-{\alpha}_k) (y_{k-1} - x_{k-1}) + (\lambda_{k-1} - \beta_{k-1}) G_{\lambda_{k-1}}(x_{k-1}, \nabla f(z_{k-1})). 
	\end{align}
	Dividing both sides by ${\Gamma}_k$ and noting that $\frac{1-{\alpha}_k}{{\Gamma}_k} = \frac{1}{{\Gamma}_{k-1}}$, we further obtain that
	\begin{align}
	\frac{y_k - x_k}{{\Gamma}_k} &= \frac{y_{k-1} - x_{k-1}}{{\Gamma}_{k-1}} + \frac{\lambda_{k-1} - \beta_{k-1}}{{\Gamma}_k} G_{\lambda_{k-1}}(x_{k-1}, \nabla f(z_{k-1})). 
	\end{align}
	Telescoping the above equality over the iterations $Q_{t-1},...,k$ { within this restart period}, noting that $x_{Q_{t-1}}=y_{Q_{t-1}}$ by restart and  rearranging, we obtain that
	\begin{align}
	\|y_k - x_k \|^2 &= \|{\Gamma}_{k} \sum_{\ell=Q_{t-1}}^{k-1} \frac{\lambda_{\ell} - \beta_{\ell}}{{\Gamma}_{\ell+1}} G_{\lambda_{\ell}}(x_{\ell}, \nabla f(z_{\ell}))\|^2 \nonumber \\
	&= \|{\Gamma}_{k} \sum_{\ell=Q_{t-1}}^{k-1} \frac{{\alpha}_{\ell+1}}{{\Gamma}_{\ell+1}} \frac{\lambda_{\ell} - \beta_{\ell}}{{\alpha}_{\ell+1}} G_{\lambda_{\ell}}(x_{\ell}, \nabla f(z_{\ell}))\|^2 \nonumber \\
	&\overset{(i)}{\le} {\Gamma}_{k} \sum_{\ell=Q_{t-1}}^{k-1} \frac{{\alpha}_{\ell+1}}{{\Gamma}_{\ell+1}} \frac{(\lambda_{\ell} - \beta_{\ell})^2}{{\alpha}_{\ell+1}^2}  \|G_{\lambda_{\ell}}(x_{\ell}, \nabla f(z_{\ell}))\|^2 \nonumber \\
	&= {\Gamma}_{k} \sum_{\ell=Q_{t-1}}^{k-1} \frac{(\lambda_{\ell} - \beta_{\ell})^2}{{\Gamma}_{\ell+1}{\alpha}_{\ell+1}}  \|G_{\lambda_{\ell}}(x_{\ell}, \nabla f(z_{\ell}))\|^2, \label{eq: 1}
	\end{align}
	where (i) uses the facts that $\{{\Gamma}_k\}_k$ is a decreasing sequence within one restart period, $\sum_{\ell=Q_{t-1}}^{k-1} \frac{{\alpha}_{\ell+1}}{{\Gamma}_{\ell+1}} = \frac{1}{{\Gamma}_k}$ for all $k\le Q_t-1$ and Jensen's inequality.
	
	We also need the following lemma, which was established as Lemma 1 and Proposition 1 in \cite{Ghadimi2016}.
	\begin{lemma}(Lemma 1 and Proposition 1, \cite{Ghadimi2016})\label{aux: 4}
		Let $g$ be a proper and closed convex function. Then, for all $u, v, x\in \mathbb{R}^d$ and $\eta>0$, the following statements hold:
		\begin{align*}
		&\inner{u}{G_{\eta}(x,u)} \ge \|G_{\eta}(x,u)\|^2 + \frac{1}{\eta} \big(g(\mathrm{prox}_{\eta g}(x-\eta u)) - g(x) \big), \\
		&\|G_{\eta}(x,u) - G_{\eta}(x,v)\| \le \|u-v\|.
		\end{align*}
	\end{lemma}

	Next, we further bound the function value gap $F(x_k)-F(x_{k-1})$ of iteration $k$ {within this restart period}. By the Lipschitz continuity of $\nabla f$ in item 3 of \Cref{assum: f+g}, we obtain that 
	\begin{align}
	f(x_k) &\le f(x_{k-1}) + \inner{\nabla f(x_{k-1})}{x_k - x_{k-1}} + \frac{L}{2}\|x_k - x_{k-1}\|^2 \nonumber \\
	&= f(x_{k-1}) + \inner{\nabla f(x_{k-1})}{- \lambda_{k-1} G_{\lambda_{k-1}}(x_{k-1}, \nabla f(z_{k-1}))} + \frac{L\lambda_{k-1}^2}{2}\|G_{\lambda_{k-1}}(x_{k-1}, \nabla f(z_{k-1}))\|^2 \nonumber \\
	&= f(x_{k-1}) - \lambda_{k-1} \inner{\nabla f(x_{k-1})-\nabla f(z_{k-1})}{G_{\lambda_{k-1}}(x_{k-1}, \nabla f(z_{k-1}))} \nonumber\\
	&\quad-  \lambda_{k-1} \inner{\nabla f(z_{k-1})}{G_{\lambda_{k-1}}(x_{k-1}, \nabla f(z_{k-1}))} 
	+ \frac{L\lambda_{k-1}^2}{2}\|G_{\lambda_{k-1}}(x_{k-1}, \nabla f(z_{k-1}))\|^2 \nonumber\\
	&\overset{(i)}{\le} f(x_{k-1}) - \lambda_{k-1} \inner{\nabla f(x_{k-1})-\nabla f(z_{k-1})}{G_{\lambda_{k-1}}(x_{k-1}, \nabla f(z_{k-1}))} -  \lambda_{k-1} \|G_{\lambda_{k-1}}(x_{k-1}, \nabla f(z_{k-1}))\|^2  \nonumber\\ 
	&\quad - \big(g(\mathrm{prox}_{\lambda_{k-1} g}(x_{k-1}-\lambda_{k-1} \nabla f(z_{k-1}))) - g(x_{k-1}) \big) + \frac{L\lambda_{k-1}^2}{2}\|G_{\lambda_{k-1}}(x_{k-1}, \nabla f(z_{k-1}))\|^2 \nonumber\\
	&= f(x_{k-1}) - \lambda_{k-1} \inner{\nabla f(x_{k-1})-\nabla f(z_{k-1})}{G_{\lambda_{k-1}}(x_{k-1}, \nabla f(z_{k-1}))} -  \lambda_{k-1} \|G_{\lambda_{k-1}}(x_{k-1}, \nabla f(z_{k-1}))\|^2  \nonumber\\ 
	&\quad - \big(g(x_k) - g(x_{k-1}) \big) + \frac{L\lambda_{k-1}^2}{2}\|G_{\lambda_{k-1}}(x_{k-1}, \nabla f(z_{k-1}))\|^2, \nonumber
	\end{align}
	where (i) follows from \Cref{aux: 4}. Rearranging the above inequality and using Cauchy-Swartz inequality yields that
	\begin{align}
	F(x_k) &\le  F(x_{k-1}) - \lambda_{k-1}(1-\frac{L\lambda_{k-1}}{2}) \|G_{\lambda_{k-1}}(x_{k-1}, \nabla f(z_{k-1}))\|^2 \nonumber\\
	&\quad + \lambda_{k-1} \|\nabla f(x_{k-1})-\nabla f(z_{k-1})\| \|G_{\lambda_{k-1}}(x_{k-1}, \nabla f(z_{k-1}))\|. \label{eq: 15}
	\end{align}
	
	Also, note that
	\begin{align}
	\|\nabla f(x_{k-1}) - \nabla f(z_{k-1})\| &\le L\|x_{k-1} - z_{k-1}\| \overset{(i)}{\le} L(1-{\alpha}_k) \|y_{k-1} - x_{k-1}\| \nonumber,
	\end{align}
	where (i) follows from the update rule of the momentum scheme. Substituting the above inequality into \cref{eq: 15} yields that
	\begin{align}
	F(x_k) &\le F(x_{k-1}) - \lambda_{k-1}(1-\frac{L\lambda_{k-1}}{2})\|G_{\lambda_{k-1}}(x_{k-1}, \nabla f(z_{k-1}))\|^2 \nonumber\\
	&\quad+ L\lambda_{k-1}(1-{\alpha}_k) \|G_{\lambda_{k-1}}(x_{k-1}, \nabla f(z_{k-1}))\|\|y_{k-1} - x_{k-1}\| \nonumber\\
	&\le F(x_{k-1}) - \lambda_{k-1}(1-\frac{L\lambda_{k-1}}{2})\|G_{\lambda_{k-1}}(x_{k-1}, \nabla f(z_{k-1}))\|^2 \nonumber\\
	&\quad+ \frac{L\lambda_{k-1}^2}{2} \|G_{\lambda_{k-1}}(x_{k-1}, \nabla f(z_{k-1}))\|^2 + \frac{L(1-{\alpha}_k)^2}{2}\|y_{k-1} - x_{k-1}\|^2 \nonumber\\
	&= F(x_{k-1}) - \lambda_{k-1}(\frac{1}{2}-L\lambda_{k-1}) \|G_{\lambda_{k-1}}(x_{k-1}, \nabla f(z_{k-1}))\|^2 + \frac{L(1-{\alpha}_k)^2}{2}\|y_{k-1} - x_{k-1}\|^2 \nonumber\\
	&\le  F(x_{k-1}) - \lambda_{k-1}(\frac{1}{2}-L\lambda_{k-1}) \|G_{\lambda_{k-1}}(x_{k-1}, \nabla f(z_{k-1}))\|^2 \nonumber\\
	&\quad+ \frac{L{\Gamma}_{k-1}}{2}\sum_{\ell=Q_{t-1}}^{k-2} \frac{\lambda_{\ell} - \beta_{\ell}}{{\alpha}_{\ell+1} {\Gamma}_{\ell+1}} \|G_{\lambda_{\ell}}(x_{\ell}, \nabla f(z_{\ell}))\|^2, \label{eq: 12}
	\end{align}
	where the last inequality uses \cref{eq: 1} and the fact that $0<{\alpha}_k <1$. Next, telescoping the above inequality over the iterations $Q_{t-1},...,k$ { within this restart period}, we further obtain that 
\begin{align}
	F(x_k) &\le F(x_{Q_{t-1}}) - \sum_{j=Q_{t-1}}^{k-1} \lambda_{j}(\frac{1}{2}- L\lambda_{j}) \|G_{\lambda_{j}}(x_{j}, \nabla f(z_{j}))\|^2 \nonumber\\
	&\quad + \sum_{j=Q_{t-1}}^{k-1} \frac{L{\Gamma}_{j}}{2} \sum_{\ell=Q_{t-1}}^{j-1} \frac{(\lambda_{\ell} - \beta_{\ell})^2}{{\Gamma}_{\ell+1}{\alpha}_{\ell+1}}  \|G_{\lambda_{\ell}}(x_{\ell}, \nabla f(z_{\ell}))\|^2  \nonumber\\
	&= F(x_{Q_{t-1}}) - \sum_{j=Q_{t-1}}^{k-1} \lambda_{j}(\frac{1}{2}- L\lambda_{j}) \|G_{\lambda_{j}}(x_{j}, \nabla f(z_{j}))\|^2 \nonumber\\
	&\quad+ \frac{L}{2}  \sum_{\ell=Q_{t-1}}^{k-1} \frac{(\lambda_{\ell} - \beta_{\ell})^2}{{\Gamma}_{\ell+1}{\alpha}_{\ell+1}}  \|G_{\lambda_{\ell}}(x_{\ell}, \nabla f(z_{\ell}))\|^2 (\sum_{j=\ell-1}^{k-1} {\Gamma}_{j}) \nonumber\\
	&\overset{(i)}{\le}  F(x_{Q_{t-1}}) - \sum_{j=Q_{t-1}}^{k-1} \lambda_{j}(\frac{1}{2}- L\lambda_{j}) \|G_{\lambda_{j}}(x_{j}, \nabla f(z_{j}))\|^2 \nonumber\\
	&\quad+ \frac{L}{2}  \sum_{\ell=Q_{t-1}}^{k-1} \frac{2(\lambda_{\ell} - \beta_{\ell})^2}{(\ell-Q_{t-1}-1) {\Gamma}_{\ell+1}{\alpha}_{\ell+1}}  \|G_{\lambda_{\ell}}(x_{\ell}, \nabla f(z_{\ell}))\|^2 \nonumber\\
	&= F(x_{Q_{t-1}}) - \sum_{j=Q_{t-1}}^{k-1} \bigg[\lambda_{j}(\frac{1}{2}- L\lambda_{j}) - \frac{L(\lambda_{j} - \beta_{j})^2}{(j-Q_{t-1}-1) {\Gamma}_{j+1}{\alpha}_{j+1}} \bigg] \|G_{\lambda_{j}}(x_{j}, \nabla f(z_{j}))\|^2 \nonumber\\
	&\overset{(ii)}{\le} F(x_{Q_{t-1}}) - \sum_{j=Q_{t-1}}^{k-1} \big[\frac{\lambda_{j}}{4} - \frac{L{\alpha}_{j+1} \beta_{j}^2}{(j-Q_{t-1}-1) {\Gamma}_{j+1}} \big] \|G_{\lambda_{j}}(x_{j}, \nabla f(z_{j}))\|^2 \nonumber\\
	&\le F(x_{Q_{t-1}}) - \sum_{j=Q_{t-1}}^{k-1} \big[\frac{\beta_{j}}{4} - \frac{\beta_{j}}{8} \big] \|G_{\lambda_{j}}(x_{j}, \nabla f(z_{j}))\|^2 \nonumber\\
	&\le F(x_{Q_{t-1}}) - \sum_{j=Q_{t-1}}^{k-1} \frac{1}{64L\lambda_{j}^2} \|x_{j+1} - x_j\|^2 \nonumber\\
	&\le F(x_{Q_{t-1}}) - \sum_{j=Q_{t-1}}^{k-1} \frac{L}{4} \|x_{j+1} - x_j\|^2, \label{eq: 8}
\end{align}

where (i) follows from the fact that $\sum_{j=\ell-1}^{k-1} {\Gamma}_{j} = 2\sum_{j=\ell-1}^{k-1} \frac{1}{j-Q_{t-1}} - \frac{1}{j-Q_{t-1}+1} \le \frac{2}{\ell-Q_{t-1}-1}$, and (ii) uses the facts that $L\lambda_{j} \le 2L\beta_j \le \frac{1}{4}$, $\lambda_{j}-\beta_{j} \le {\alpha}_{j+1} \beta_{j}$. Then, setting $k$ in the above inequality to be the last iteration $Q_t-1$ within this restart period and note that $x_{Q_t} = x_{Q_t-1}$, we obtain that
\begin{align}
	F(x_{Q_t}) &\le  F(x_{Q_{t-1}}) - \frac{L}{4}\sum_{k=Q_{t-1}}^{Q_t-1} \|x_{k+1} - x_k\|^2. \label{eq: 7}
\end{align}

The first inequality is proved.

To prove the second inequality, by the optimality condition of the proximal gradient update for $x_{k}$, we obtain that
\begin{align}
-\nabla f(z_{k-1}) - \frac{1}{\lambda_k}(x_{k}-x_{k-1}) \in \partial g(x_{k}), \nonumber
\end{align}
which further implies that
\begin{align}
\nabla f(x_{k})-\nabla f(z_{k-1}) - \frac{1}{\lambda_{k-1}}(x_{k}-x_{k-1}) \in \partial F(x_{k}). \nonumber
\end{align}
Note that $\dist_{\partial F(x_{k})}(\zero) \le u_k$ for any $u_k \in \partial F(x_{k})$. Therefore, the above inequality further implies that
\begin{align}
\dist_{\partial F(x_{k})}(\zero) &\le \|\nabla f(x_{k})-\nabla f(z_{k-1}) - \frac{1}{\lambda_{k-1}}(x_{k}-x_{k-1})\| \nonumber\\
&\le  \|\nabla f(x_{k})- \nabla f(x_{k-1})\| + \|\nabla f(x_{k-1}) -\nabla f(z_{k-1})\| + \frac{1}{\lambda_{k-1}} \|x_{k}-x_{k-1}\| \nonumber\\
&\overset{(i)}{\le} 9L \|x_k - x_{k-1}\| + L \sqrt{{\Gamma}_{k-1} \sum_{\ell=Q_{t-1}}^{k-2} \frac{(\lambda_{\ell} - \beta_{\ell})^2}{{\Gamma}_{\ell+1}{\alpha}_{\ell+1}}  \|G_{\lambda_{\ell}}(x_{\ell}, \nabla f(z_{\ell}))\|^2}, \label{eq: 13}
\end{align}
where (i) uses the Lipschitz gradient property, the update rule of \Cref{alg: Acc-PGD} and \cref{eq: 1}. Squaring both sides of the above inequality and rearranging, we further obtain that
\begin{align}
\dist_{\partial F(x_{k})}^2(\zero) &\le 162L^2 \|x_k - x_{k-1}\|^2 + 2L^2{\Gamma}_{k-1} \sum_{\ell=Q_{t-1}}^{k-2} \frac{(\lambda_{\ell} - \beta_{\ell})^2}{{\Gamma}_{\ell+1}{\alpha}_{\ell+1}}  \|G_{\lambda_{\ell}}(x_{\ell}, \nabla f(z_{\ell}))\|^2 \nonumber\\
&\le 162L^2 \|x_k - x_{k-1}\|^2 + 2L^2{\Gamma}_{k-1} \sum_{\ell=Q_{t-1}}^{k-2} \frac{{\alpha}_{\ell+1} \beta_{\ell}^2}{{\Gamma}_{\ell+1} \lambda_{\ell}^2}  \|x_{\ell+1} - x_{\ell}\|^2 \nonumber\\
&\le 162L^2 \|x_k - x_{k-1}\|^2 + 2L^2{\Gamma}_{k-1} \sum_{\ell=Q_{t-1}}^{k-2} \frac{{\alpha}_{\ell+1} }{{\Gamma}_{\ell+1}}  \|x_{\ell+1} - x_{\ell}\|^2 \nonumber\\
&\le 162L^2 \|x_k - x_{k-1}\|^2 + 2L^2\frac{2}{(k-Q_t-1)(k-Q_t-2)} \sum_{\ell=Q_{t-1}}^{k-2} (\ell+1-Q_t)  \|x_{\ell+1} - x_{\ell}\|^2 \nonumber\\
&\le 162L^2 \sum_{\ell=Q_{t-1}}^{k-1} \|x_{\ell+1} - x_{\ell}\|^2. \nonumber
\end{align}
Then, set $k$ in the above inequality to be the last iteration $Q_t-1$ within this restart period and note that $x_{Q_t} = x_{Q_t-1}$, we obtain that
\begin{align}
\dist_{\partial F(x_{Q_t})}^2(\zero) \le 162L^2 \sum_{k=Q_{t-1}}^{Q_t-1} \|x_{k+1} - x_{k}\|^2. \nonumber
\end{align}
The second inequality is proved.

\end{proof}

\section{Proof of \Cref{thm: global}}

\TheoremGlobal*

\begin{proof}
	Consider any iteration $K$ and the corresponding closet restart checkpoint $Q_t$ (for some $t$). In the proof of \Cref{lemma: Acc-PGD dynamic}, we have shown that (see \cref{eq: 8})
	\begin{align}
	F(x_{K}) &\le  F(x_{Q_{t}}) - \frac{L}{4}\sum_{j=Q_{t}}^{K-1} \|x_{j+1} - x_j\|^2. \label{eq: 11}
	\end{align}
	On the other hand, by \Cref{lemma: Acc-PGD dynamic} we know that for all $\ell=1,..., t$,
	\begin{align}
	F(x_{Q_\ell}) &\le  F(x_{Q_{\ell-1}}) - \frac{L}{4}\sum_{k=Q_{\ell-1}}^{Q_{\ell}-1} \|x_{k+1} - x_k\|^2.
	\end{align}
	Telescoping the above inequality over $\ell=1,..., t$ and combining with \cref{eq: 11}, and noting that $Q_0=q_0=0$, $x_{Q_\ell} = x_{Q_{\ell}-1}$ for all $\ell$, we obtain that
	\begin{align*}
	F(x_{K}) &\le  F(x_{0}) - \frac{L}{4}\sum_{j=0}^{K-1} \|x_{j+1} - x_j\|^2 = F(x_{0}) - \frac{L}{4}\sum_{j=0}^{K-1} \lambda_{j}^2 \|G_{\lambda_j}(z_j, \nabla f(z_j))\|^2.
	\end{align*}
	Note that $\lambda_j > \beta_{j} = \frac{1}{8L}$. Then, the above inequality further implies that
	\begin{align*}
	\frac{1}{256L}\sum_{j=0}^{K-1} \|G_{\lambda_j}(z_j, \nabla f(z_j))\|^2 \le  F(x_{0}) - F(x_{K}) \le F(x_{0}) - F^*.
	\end{align*}
	Ignoring the universal constants in the above inequality and taking the minimum, we obtain that
	\begin{align*}
	\min_{0\le k\le K-1}\|G_{\lambda_k}(z_k, \nabla f(z_k))\|^2 \le \Theta\bigg({\frac{L\big(F(x_{0}) - F^*\big)}{K}}\bigg).
	\end{align*}
	
\end{proof}

\section{Proof of \Cref{thm: Acc-GD variable}}

\TheoremVariable*

\begin{proof}
	Recall that the length of the iteration path of the $t$-th restart period is defined as
	\begin{align}
	L_t:= \sqrt{\sum_{k=Q_t}^{Q_{t+1}-1} \|x_{k+1}-x_k\|^2}.
	\end{align}
	Then, we can rewrite the results of \Cref{lemma: Acc-PGD dynamic} as
	\begin{align}
	F(x_{Q_t}) &\le  F(x_{Q_{t-1}}) - \frac{L}{4}L_{t-1}^2, \label{eq: 2}\\
	\dist_{\partial F(x_{Q_t})}^2(\zero) &\le 162L^2 L_{t-1}^2.\label{eq: 3}
	\end{align}
	By \cref{eq: 2}, the function value sequence $\{F(x_{Q_t}) \}_t$ decreases monotonically period-wise.  Since the objective function $F$ is bounded below (item 1 of \Cref{assum: f+g}), we conclude that $\{F(x_{Q_t})\}_t$ converges to a certain finite limit $F^*$. Also, since $F$ has bounded sub-level sets (item 2 of \Cref{assum: f+g}), \cref{eq: 2} further implies that the sequence $\{x_{Q_t} \}_t$ is bounded. 
	
	The above proof shows that $F(x_{Q_t}) \downarrow F^*$ and $\{x_{Q_t}\}_t$ is bounded. Next, we further show that the entire sequences $\{F(x_{k})\}_k, \{x_k\}_k$ share the same properties. Telescoping \cref{eq: 2} over $t=1,2,...T$ yields that: for any $T\in \mathbb{N}$,
	\begin{align}
	\sum_{t=0}^{T-1} L_{t}^2 \le L(F(x_0) - F(x_{Q_T})) \le L(F(x_0) - \inf_{x\in \mathbb{R}^d} F(x) ) < +\infty.
	\end{align}
	Letting $T\to \infty$ we conclude that $\sum_{t=0}^{\infty} L_{t}^2 < +\infty$ and therefore $L_t \overset{t}{\to} 0$.
	Since each restart period contains a uniformly bounded number of iterations, this further implies that $\lim_{k\to \infty} \|x_{k+1} - x_k\| = 0$. Therefore, the entire sequence $\{x_k \}_k$ is bounded and we denote $\omega$ as its set of limit points ($\omega$ is a compact set). Also, by the facts that $\lim_{k\to \infty} \|x_{k+1} - x_k\| = 0$ and \cref{eq: 12}, we conclude that $\lim_{k\to \infty} F(x_{k+1}) - F(x_k) = 0$ for all $k\in \mathbb{N}$. Since $F(x_{Q_t}) \downarrow F^*$, we conclude that $F(x_k) \to F^*$. To this end, we have shown that the entire sequence $\{x_k \}_k$ has a limit point set $\omega$ and the entire sequence $\{F(x_k) \}_k$ converges to a certain finite limit $F^*$.

	Now consider any limit point $x^*\in \omega$ and without loss of ambiguity we assume that $x_{k} \overset{k}{\to} x^*$ along a proper subsequence. By the proximal gradient update step of $x_k$ we obtain that
	\begin{align}
	g(x_{k}) + \frac{1}{2\lambda_{k-1}} \|x_k - x_{k-1}\|^2 &+ \inner{\nabla f(z_{k-1})}{x_k - x_{k-1}} \nonumber\\ 
	&\le  g(x^*) + \frac{1}{2\lambda_{k-1}} \|x^* - x_{k-1}\|^2 + \inner{\nabla f(z_{k-1})}{x^* - x_{k-1}}. \nonumber
	\end{align} 
	Taking limsup on both sides of the above inequality and noting that $\{x_k\}_k$ is bounded, $\|x_k - x_{k-1}\| \to 0$ and $x_k \to x^*$, we conclude that  $\limsup_k g(x_{k}) \le g(x^*)$. Since $g$ is lower-semicontinuous, we know that $\limsup_k g(x_{k}) \ge g(x^*)$. Combining these two inequalities yields that $\lim_k g(x_{k}) = g(x^*)$. By continuity of $f$, we further conclude that $\lim_k F(x_{k}) = F(x^*)$. Since we have shown that the entire sequence $\{F(x_{k})\}_k$ converges to a certain finite limit $F^*$, we conclude that $F(x^*)\equiv F^*$ for all $x^*\in \omega$. Also, \cref{eq: 13} and the fact that $\|x_{k+1} - x_k\| \to 0$ further imply that $\dist_{\partial F(x_{k})}(\zero) \overset{k}{\to} 0$.     
	To this end, we have shown that for every subsequence $x_{k} \to x^* \in \omega$ we have $F(x_{k}) \to F(x^*)$ and $\dist_{\partial F(x_{k})}(\zero)  \to 0$. Recall the definition of limiting sub-differential, we conclude that every limit point $x^*$ of $\{x_k\}_k$ is a critical point, i.e., $\zero\in \partial F(x^*)$. 	
	
	Next, we show that the sequence $\{x_k\}_k$ has a unique limit point under the \KL property. 
	Consider any limit point $x^*\in \omega$. We have shown that 1) $F(x^*)\equiv F^*$ for all $x^*\in\omega$; 2)
	$F(x_{Q_t}) \downarrow F^*$; and 3) $\dist_{\partial F(x_{k})}(\zero)  \to 0$. Collecting these  facts, we are ready to apply the K{\L} property for $t$ being sufficiently large. Specifically, by the K{\L} property of the objective function, we obtain that: for all $t\ge t_1$ where $t_1$ is a sufficiently large integer, 
	\begin{align}
		\varphi'(F(x_{Q_t}) - F^*) \ge \frac{1}{\dist_{\partial F(x_{Q_t})}(\zero)} \overset{(i)}{\ge} \frac{1}{15 L \cdot L_{t-1}}, \label{eq: 4}
	\end{align}
	where (i) follows from \cref{eq: 3}. Then, by concavity of $\varphi$ and \cref{eq: 2,eq: 4}, we further obtain that
	\begin{align}
		\varphi(F(x_{Q_t}) - F^*) - \varphi(f(x_{Q_{t+1}}) - F^*) &\ge \varphi'(F(x_{Q_t}) - F^*) (F(x_{Q_t}) - F(x_{Q_{t+1}})) \nonumber\\
		&\ge \frac{L_t^2}{60L^2 \cdot L_{t-1}}. \label{eq: 5}
	\end{align}
	Rearranging the above inequality yields that 
	\begin{align}
		L_t^2 \le 60L^2L_{t-1} \big[\varphi(F(x_{Q_t}) - F^*) - \varphi(F(x_{Q_{t+1}}) - F^*) \big]. \nonumber
	\end{align}
	Taking square root of both sides of the above inequality and using the fact that $\sqrt{ab} \le \frac{a+b}{2}$ for $a,b>0$, we obtain that
	\begin{align}
		2L_t \le L_{t-1} + 60L^2\big[\varphi(F(x_{Q_t}) - F^*) - \varphi(F(x_{Q_{t+1}}) - F^*) \big].
	\end{align}
	Telescoping the above inequality over $t=t_1+1,...T$ yields that 
	\begin{align}
		2\sum_{t=t_1+1}^T L_t &\le \sum_{t=t_1+1}^T L_t + L_{t_1} + 60L^2\big[\varphi(F(x_{Q_{t_1+1}}) - F^*) - \varphi(F(x_{Q_{T+1}}) - F^*) \big] \nonumber\\
		&\le \sum_{t=t_1+1}^T L_t + L_{t_1} + 60L^2\varphi(F(x_{Q_{t_1+1}}) - F^*), \nonumber
	\end{align}
	where the last inequality follows from the fact that $F(x_{Q_t}) \ge F^*$ for all $t\ge t_1$ and $\varphi(s)>0$ for all $s>0$. Rearranging the above inequality yields that: for all $T \ge t_1$
	\begin{align}
	\sum_{t=t_1+1}^T L_t &\le L_{t_1} + 60L^2\varphi(F(x_{Q_{t_1+1}}) - F^*)<+\infty. \nonumber
	\end{align}
	Letting $T\to \infty$ and noting that $t_1$ is a finite integer, we finally conclude that
	\begin{align}
	\sum_{t=0}^\infty L_t < +\infty. \nonumber
	\end{align}
	To further prove the convergence of the variable sequence, note that $L_t := \sqrt{\sum_{k=Q_t}^{Q_{t+1}-1} \|x_{k+1}-x_k\|^2}\ge \frac{1}{\sqrt{Q_{t+1}-Q_t}} \sum_{k=Q_t}^{Q_{t+1}-1} \|x_{k+1}-x_k\|$. Substituting into the above inequality yields that
	\begin{align}
	\sum_{t=0}^\infty \frac{1}{\sqrt{Q_{t+1}-Q_t}} \sum_{k=Q_t}^{Q_{t+1}-1} \|x_{k+1}-x_k\| \le \max_t \frac{1}{\sqrt{Q_{t+1}-Q_t}} \sum_{k=0}^\infty \|x_{k+1}-x_k\|< +\infty, \nonumber
	\end{align}
	where the last inequality uses the fact that all restart periods have uniformly bounded numbers of iterations that are uniformly bounded. 
	Therefore, the sequence $\{\|x_{k+1}-x_k\| \}_k$ is absolutely summable and this implies that $\{x_k \}_k$ is a convergent Cauchy sequence. Since we have shown that all the limit points of $\{x_k \}_k$ are critical points, we conclude that $\{x_k \}_k$ converges to a certain critical point of $F$. Lastly, it is clear from the previous results that $\|x_k-y_k\|\to 0, \|x_k-z_k\|\to 0$, which imply that both $\{y_k\}_k$ and $\{z_k\}_k$ converge to the same limit.
	
\end{proof}

\section{Proof of \Cref{thm: Acc-GD rates} and \Cref{thm: Acc-GD var_rates}}
\TheoremRates*

\TheoremRatesVariable*

\begin{proof}
	Consider any $t$-th restart period and denote $r_t:= F(x_{Q_t}) - F(x^*)$ as the function value gap. Then, we can rewrite \cref{eq: 5} as: for all sufficiently large $t\ge t_0$,
	\begin{align}
		60L^2\big(\varphi(r_t) - \varphi(r_{t+1}) \big) \ge \frac{L_t^2}{L_{t-1}}.
	\end{align}
	
	Next, fix $\gamma \in (0,1)$ and consider any $t\ge t_0$. Suppose that $L_t\ge \gamma L_{t-1}$, then the above inequality implies that
	\begin{align}
		L_t \le \frac{60L^2}{\gamma^2} \big(\varphi(r_t) - \varphi(r_{t+1}) \big).
	\end{align}
	Otherwise, we conclude that $L_t\le \gamma L_{t-1}$. Combining these two inequalities yields that
	\begin{align}
		L_t \le \gamma L_{t-1} + \frac{60L^2}{\gamma^2} \big(\varphi(r_t) - \varphi(r_{t+1}) \big).
	\end{align}
	Summing the above inequality over $t=t_0,...,T$ yields that
	\begin{align}
	\sum_{t=t_0}^{T} L_t &\le \gamma \sum_{t=t_0}^{T}L_{t-1} + \frac{60L^2}{\gamma^2} \big(\varphi(r_{t_0}) - \varphi(r_{T+1}) \big) \nonumber\\
	&\le \gamma \Big[\sum_{t=t_0}^{T}L_{t} + L_{t_0-1} \Big] + \frac{60L^2}{\gamma^2} \varphi(r_{t_0}). \nonumber
	\end{align}
	Rearranging the above inequality yields that: for all $T\ge t_0$,
	\begin{align}
	\sum_{t=t_0}^{T} L_t &\le \frac{\gamma}{1-\gamma} L_{t_0-1} + \frac{60L^2}{\gamma^2(1-\gamma)} \varphi(r_{t_0}). \nonumber
	\end{align}
	Next, define $\Delta_{t_0}:= \sum_{t=t_0}^{\infty} L_t$, which is well-defined due to \cref{eq: finite_len}. Then, letting $T\to \infty$ in the above inequality and noting that $\varphi(s)=Cs^\theta$ yields that for all sufficiently large $t$
	\begin{align}
	\Delta_{t} &\le \frac{\gamma}{1-\gamma} (\Delta_{t-1} - \Delta_{t}) + \frac{CL^2}{\gamma^2(1-\gamma)} r_{t}^{\theta} \nonumber \\
	&\overset{(i)}{\le} \frac{\gamma}{1-\gamma} (\Delta_{t-1} - \Delta_{t}) + \frac{CL^{\frac{1}{1-\theta}}}{\gamma^2(1-\gamma)}  \Big[\sum_{k=(t-1)q}^{tq-1}\|x_{k+1} - x_k\|^2\Big]^{\frac{\theta}{2(1-\theta)}} \nonumber \\
	&= \frac{\gamma}{1-\gamma} (\Delta_{t-1} - \Delta_{t}) + \frac{CL^{\frac{1}{1-\theta}}}{\gamma^2(1-\gamma)} (\Delta_{t-1} - \Delta_{t})^{\frac{\theta}{1-\theta}} \nonumber \\
	\end{align}
	where (i) uses the \KL property and the dynamics of APG-restart in \Cref{lemma: Acc-PGD dynamic}, i.e., $r_{t} \le C\dist_{\partial F(x_{Q_t})}^{\frac{1}{1-\theta}}(\zero) \le C \Big[L^2 \sum_{k=Q_{t-1}}^{Q_t-1}\|x_{k+1} - x_k\|^2\Big]^{\frac{1}{2(1-\theta)}}$. It has been shown in (Attouch \& Bolte 09) that sequence $\{\Delta_t\}_t$ satisfying the above inductive property converges to zero at different rates depending on $\theta$ as stated in the theorem. Finally, we note that Holder's inequality and triangle inequality imply that $\max_t \frac{1}{\sqrt{Q_{t+1}-Q_t}}\|x_{Q_t} - x^*\| \le \Delta_t$, and the result follows.

	To prove the convergence rates of the function value gap, consider any $t$-th restart period and denote $r_t:= F(x_{Q_t}) - F(x^*)$ as the function value gap. As we have shown that $r_t \overset{t}{\to} 0$, for sufficiently large $t$ we can apply the \KL property and obtain that: for some universal constant $C>0$,
	\begin{align}
		r_t &\le C\dist_{\partial F(x_{Q_t})}^{\frac{1}{1-\theta}}(\zero) = C\sqrt{\dist_{\partial F(x_{Q_t})}^{\frac{1}{1-\theta}}(\zero)} \nonumber\\
		&\overset{(i)}{\le} C\sqrt{\Big(L^2\sum_{k=Q_{t-1}}^{Q_t-1} \|x_{k+1} - x_{k}\|^2 \Big)^{\frac{1}{1-\theta}}} \nonumber\\
		&\overset{(ii)}{\le} CL^{\frac{3}{2(1-\theta)}} \big(r_{t-1} -r_t \big)^{\frac{1}{2(1-\theta)}}, \nonumber
	\end{align}
where the constant $C$ may vary from line to line in the above derivation, (i) and (ii) follow from \Cref{lemma: Acc-PGD dynamic}. Rearranging the above inequality yields that: for all sufficiently large $t$,	
\begin{align}
	1\le CL^3r_t^{2(\theta -1)} (r_{t-1} - r_t). \nonumber
\end{align}
It has been shown in (Frankel et al., 2015; Li \& Lin, 2015) that sequence $\{r_t\}_t$ satisfying the above inductive property converges to zero at different rates depending on $\theta$ as stated in the theorem.	
\end{proof}

\section{Restart Conditions Used in the Experiments}\label{app: exp}
\begin{enumerate}
	\item For the fixed restart scheme we set the restart period to be $q=10,30,50$, respectively;
	\item For the function scheme, we relax the condition to be
	\begin{align*}
		F(x_k) > 0.8F(x_{k-1}).
	\end{align*}
	\item For the gradient mapping scheme, we relax the condition to be
	\begin{align*}
	\inner{z_{k}-y_{k}}{y_{k+1}-z_{k}} \ge -0.2 \|z_{k}-y_{k}\|\|y_{k+1}-z_{k}\|.
	\end{align*}
	\item For the non-monotone scheme, we relax the condition to be
	\begin{align*}
	\inner{z_{k}-y_{k}}{y_{k+1}-\frac{z_{k}+x_k}{2}} \ge -0.2\|z_{k}-y_{k}\|\Big\|y_{k+1}-\frac{z_{k}+x_k}{2}\Big\|.
	\end{align*}
\end{enumerate}
